# Supplementary material for: How Effective Are They? Exploring Large Language Model Based Fuzz Driver Generation
Source: arXiv:2307.12469 source file (2024-07-29)
Supplement: Supplementary file 1 [file 10-appendix.tex]

\section{Details of Proposed Fix Prompt Templates}
\label{sec:fix-templates-detail}
Table~\ref{tab:fix-templates-detail} lists the detailed design of seven prompt templates used for fixing seven types of failures.
Concrete examples can be found in ~\cite{fuzz-drvier-study-website}.

\section{Detail of Quiz Questions}
\label{sec:quiz-questions-detail}
Table~\ref{tab:quiz} shows the full list of the 86 questions included in our quiz.

\section{Full List of Evaluation Results for All Query Strategies}
\label{sec:evaluation-results-full-list}
Table~\ref{tab:eval_full} posts the detailed statistics of evaluation results.

\onecolumn

\begin{table*}[h]
\caption{Detail of Different Fix Prompt Templates.}
\label{tab:fix-templates-detail}
\resizebox{0.9\textwidth}{!}{
% [inline block 0: 18 envs, 92217 chars -> data_tex | \begin{tabular}{ll} \toprule...]


}
\end{table*}
